# Supplementary material for: Topological invariant responsible for the stability of the Fermi surfaces in non-homogeneous systems
Source: arXiv:2508.20772 source file (2025-10-05)
Supplement: Supplementary file 1 [file N3_JETP_supplementary_07_09_25_cor.tex]

\documentclass[aps,prd,showpacs,twocolumn,nofootinbib,superscriptaddress]{revtex4-2}
\usepackage{amsmath,amssymb,amsfonts}
\usepackage{bm}
\usepackage{verbatim}
\usepackage{hyperref}
\usepackage{slashed,braket}
\usepackage{ulem}
\usepackage{cancel}
\usepackage{color}
\usepackage{graphicx,graphics}
\usepackage[title,titletoc]{appendix}
\usepackage{stackengine}
\usepackage{mathrsfs}
\usepackage{tikz-feynman}
\usepackage{amsthm}

\usepackage{tikz}
\usepackage{pgfplots}
%\pgfplotsset{compat=1.18}

\usepackage{lineno}
%\linenumbers
\usepackage[T1]{fontenc} % if needed
\usepackage{braket}

\usepackage{bbold}
\usepackage{comment}
\excludecomment{confidential}
\usepackage{makecell}
\usepackage{bm}
\usepackage{braket}
\usepackage{slashed}
\usepackage{mathtools}

\usepackage{amsthm}

\newcommand{\tr}{\operatorname{tr}}

\begin{document}
	
	\title{{ Supplementary Material to the article} \\ “Topological invariant responsible for the stability of the Fermi surfaces in non - homogeneous systems”}

	%\date{\today}

	%\pacs{}
	
	\maketitle
	
	%\tableofcontents
	%\section{Introduction}
	%\label{SectIntro}

In these Supplementary materials we consider examples of  the non - homogeneous systems with nontrivial $N_3^{(T)}$. Our constructions are based on an analogy to the system in the presence of constant external magnetic field. We start from the particular model with $M=1$, and next consider its variations, in particular, with nontrivial matrix structure ($M>1$).

\section{Definition of the model and calculation of $N_3$}

Let us consider the non - interacting system with Dirac operator of the form
\begin{equation}
	\hat{Q} = i \kappa \hat{p}_4 \hat{p}_3 - \hat{p}_3 -  \frac{\Bigl(\hat{p}_1^2 + (\hat{p}_2 - \hat{x}_1 B)^2 \Bigr) }{2m} + \mu
\end{equation}
with parameters $\kappa$, $m$, $\mu$, and $B$. The model with the Dirac operator of this type may appear as  effective description of an interacting system (the interactions cause change of the term $p_4 \to \kappa p_4 p_3$). 
The associated quantum field theory is well defined, and the corresponding topological invariant is given by Eq. (56) of the main text. (Obviousely, in this case $\hat{T} = 1$.) It can be calculated for $p_4 = \pm \epsilon \to 0$:
$$
N_3^{} = N_3^{+\epsilon} - N_3^{-\epsilon}
$$ 
where 
\begin{eqnarray} 
	N^{\epsilon}_3&	=&{-}\frac{1}{V \,24\pi^2}\int d^3 x\int_{p_4 = \epsilon} \text{tr}_{D}\Bigl({G}_W\star d{Q}_W\nonumber\\&&\star \wedge d{G}_W\star\wedge d{Q}_W \Bigr) \label{Ni2}
\end{eqnarray}
This expression can be calculated using technique developed in \cite{zubkov2020topological}. Using this machinery we arrive at
\begin{eqnarray}
	N^{\epsilon}_3 &=& \frac{\epsilon_{ij}}{2 A}\sum_{n,k}\int dp_3\frac{1}{(p_3 + E_n - i \epsilon \kappa p_3)^2(p_3 + E_k -i \epsilon \kappa p_3)}\nonumber\\&&\langle n | [\hat{H},\hat{x}_i]|k\rangle \langle k | [\hat{H},\hat{x}_j]|n\rangle 
\end{eqnarray}
with 
\begin{equation}
	\hat{H} = \frac{\Bigl(\hat{p}_1^2 + (\hat{p}_2 - \hat{x}_1 B)^2 \Bigr) }{2m} - \mu, \quad \hat{H}|n\rangle = E_n |n\rangle
\end{equation}
At $\epsilon  \to \pm 0$ we can also represent the above expression as 
\begin{eqnarray}
&&	N^{\epsilon}_3 = \frac{\epsilon_{ij}}{2 A}\sum_{n,k}\int dp_3\langle n | [\hat{H},\hat{x}_i]|k\rangle \langle k | [\hat{H},\hat{x}_j]|n\rangle\nonumber\\&&\frac{1}{(p_3 + E_n + i \delta \, {\rm sign}\, E_n )^2(p_3 + E_k + i \delta\, {\rm sign}\, E_k )} 
\end{eqnarray}
with $\delta \to 0$.
Integrating over $p_3$ we arrive at 
\begin{eqnarray}
	N^{\epsilon}_3 &=&  2\pi i {\rm sign}\,\delta\,\frac{\epsilon_{ij}}{ A}\sum_{n,k}\int dp_3\frac{1}{(E_k - E_n )^2}\nonumber\\&&\langle n | [\hat{H},\hat{x}_i]|k\rangle \langle k | [\hat{H},\hat{x}_j]|n\rangle  \theta (-E_n)\theta(E_k)
\end{eqnarray}

This expression is similar to the one of the 2+1 D one. The result is given by 
\begin{equation}
	N_3^\epsilon = {\rm sign}\,\epsilon\,\sum_n \Theta( - E_n(B,m)),
\end{equation}
where $E_n$ is the energy of the $n$ - th Landau level 
\begin{equation}
	E_n(B,m)  = \frac{B}{m} (n+1/2) -\mu, \quad n = 0,1,...
\end{equation}
One can see that $N_3^{-\epsilon} = - N_3^{+\epsilon}$, and we arrive at 
$$
N_3^{} = 2 \Bigl[\frac{\mu - B/(2m)}{B/m}\Bigr] \theta(\mu - B/(2m))
$$
 By $\Bigl[ z \Bigr]$ we denote the integer part of $z$, i.e. the integer number that is most close to $z$ while being smaller than $z$.

\subsection{Calculation of $N_3$ for $p_4 = \omega_\pm(p_3)$}

$N_3$ can be calculated for $p_4 =  \omega_\pm(p_3)$ (we assume that $\omega_+(p_3)>0$ while $\omega_-(p_3) < 0$):
$$
N_3^{} = N_3^{\omega_+} - N_3^{\omega_-}
$$ 
where 
\begin{eqnarray} 
	N^{\omega}_3&	= &{-}\frac{1}{V \,24\pi^2}\int d^3 x\int_{p_4 = \omega} \text{tr}_{D}\Bigl({G}_W\star d{Q}_W\nonumber\\&&\star \wedge d{G}_W\star\wedge d{Q}_W \Bigr) \label{Ni20}
\end{eqnarray}
This expression can be calculated using technique developed in \cite{zubkov2020topological}. Using this machinery we arrive at
\begin{eqnarray}
	N^{\omega}_3 &=& \frac{\epsilon_{ij}}{2 A}\sum_{n,k}\int dp_3{\partial_{p_3}\Bigl(p_3 (1- i \kappa \omega(p_3)) \Bigr)}\nonumber\\&&\frac1{(p_3 + E_n - i \omega(p_3) \kappa p_3)^2(p_3 + E_k - i \omega(p_3) \kappa p_3)}\nonumber\\&&\langle n | [\hat{H},\hat{x}_i]|k\rangle \langle k | [\hat{H},\hat{x}_j]|n\rangle 
\end{eqnarray}
with 
\begin{equation}
	\hat{H} = \frac{\Bigl(\hat{p}_1^2 + (\hat{p}_2 - \hat{x}_1 B)^2 \Bigr) }{2m} - \mu, \quad \hat{H}|n\rangle = E_n |n\rangle \label{energylevels}
\end{equation}
We can easily calculate $N_3^\omega$
integrating over $p_3$:  
\begin{eqnarray}
	N^{\omega}_3 &=&  2\pi i {\rm sign}\,\omega\,\frac{\epsilon_{ij}}{ A }\sum_{n,k}\int dp_3\frac{1}{(E_k - E_n )^2}\nonumber\\&&\langle n | [\hat{H},\hat{x}_i]|k\rangle \langle k | [\hat{H},\hat{x}_j]|n\rangle  \theta (-E_n)\theta(E_k)
\end{eqnarray}

This expression is similar to the one of the 2+1 D one. The result is given by 
\begin{equation}
	N_3^\omega = {\rm sign}\,\omega\,\sum_n \Theta( - E_n(B,m)),
\end{equation}
where $E_n$ is the energy of the $n$ - th Landau level 
\begin{equation}
	E_n(B,m)  = \frac{B}{m} (n+1/2) -\mu, \quad n = 0,1,...
\end{equation}
\thispagestyle{empty}
One can see that $N_3^{\omega_-} = - N_3^{\omega_+}$, and we again arrive at 
$$
N_3^{} = 2 \Bigl[\frac{\mu - B/(2m)}{B/m}\Bigr] \theta(\mu - B/(2m))
$$

{One can see that there is no dependence of the result on the form of functions $\omega_\pm(p_3)$.}

\subsection{Wigner transformed Green function and its singularities }

First of all let us consider the Groenewold equation
$$
Q_W \star G_W = 1
$$
We have
\begin{equation}
	Q_W = i {p}_4 p_3\kappa- {p}_3 -  \frac{\Bigl({p}_1^2 + ({p}_2 - {x}_1 B)^2 \Bigr) }{2m}+\mu\label{QW1}
\end{equation}
and the Groenewold equation receives the form ($G = \bar{G}e^{2i(p_2/B - x_1)p_1)} $):
\begin{equation}
	\Bigl(B^2 \partial_{p_1}^2 + \partial_{x^1}^2  + 8m(ip_4p_3\kappa - p_3+\mu)\Bigr) \bar{G} = 8m  e^{-2i(p_2/B - x_1)p_1}\label{difeqG}
\end{equation}
Let us define the new variables
$$
z = x_1 - p_2/B, \quad q = p_1/B
$$
We arrive at
\begin{equation}
	\Bigl(\partial_{q}^2 + \partial_{z}^2 +  8m(ip_4p_3\kappa - p_3 + \mu)\Bigr) \bar{G} = 8m  e^{-2iB z q}
\end{equation}
Solution of this equation gives
\begin{eqnarray}
	&&{G}_W(x_1,p_1,p_2,p_3,p_4) =- \frac{2m}{\pi } e^{2i(p_2/B - x_1)p_1} \times \nonumber\\&&\times \int \frac{e^{-i\gamma (x_1 - p_2/B) - i \xi p_1 - i \xi \gamma/2}}{B^2\xi^2 + \gamma^2  - 8m (ip_4p_3\kappa - p_3 + \mu)}d\gamma d\xi \label{GW1}
\end{eqnarray}
At a first look expression entering Eq. (\ref{GW1}) has singularities at $p_3 = 0$ for any values of other arguments of $G_W$. However, we should take into account that the Green function of Eq. (\ref{difeqG}) is to be defined in a way that the poles in Eq. (\ref{GW1}) are to be avoided in certain way (the way to avoid the pole determines the type of the Green function). 

The situation beccomes more transparent when we consider the representation of $G_W$ through the sum over Landau levels.  The true singularities of the Green function appear if the corresponding energy levels (chemical potential included) are vanishing. Let us refine the definition of Eq.(\ref{energylevels}), and consider it with parameter $p_2$ instead of operator $\hat{p}_2$:
\begin{eqnarray}
	&&\hat{H} = \frac{\Bigl(\hat{p}_1^2 + ({p}_2 - \hat{x}_1 B)^2 \Bigr) }{2m} - \mu, \quad  \hat{H}|n, p_2\rangle = E_n |n, p_2\rangle, \nonumber\\&& \langle x_1|n, p_2\rangle = \Psi_n(x - p_2/B)
\end{eqnarray}
That is we denote by numbers $n$ the Landau levels, while these levels are degenerate (corresponding to number $p_2$). We obtain for the Green function:
\begin{eqnarray}
	&&G_W(x_1,p_1,p_2,p_3,p_4) = \sum_n \int dy e^{ip_1 y}\nonumber\\&&\frac{\Psi_n(x_1 - y/2 - p_2/B) \bar{\Psi}_n(x_1 + y/2 - p_2/B)}{ip_4 p_3 \kappa - p_3 - \frac{B}{m}(n+1/2) + \mu}
\end{eqnarray}
If $\mu$ does not coincide with either of the levels $\frac{B}{m}(n+1/2)$, the singularities of the above expresion appear at 
\begin{equation}
	p_4 = 0, \quad p_3 = \mu - \frac{B}{m}(n+1/2), n = 0, 1, ...  
\end{equation}
These are the two dimensional hypersurfaces in the hyperplane $p_4 =0$ parametrized by $p_1,p_2$. Their positions do not depend on $x$. 

\subsection{Calculation of $N^{(i)}_3$ }

Let us consider surface $\Sigma$ of the form of a collection of three - dimensional hypersurfaces $\Sigma^{(l)}$ surrounding the poles of the Green function. Each hypersurface $\Sigma^{(l)}$ has the form of a tube (small closed curve in plane $(p_4,p_3)$ surrounding the $n$ - th pole times the plane $(p_1,p_2)$). 

We obtain
\begin{eqnarray}
	&& N^{\omega_+(l)}_3 = \frac{\epsilon_{ij}}{2 A}\sum_{n,k}\int dp_3\langle n | [\hat{H},\hat{x}_i]|k\rangle \langle k | [\hat{H},\hat{x}_j]|n\rangle\nonumber\\&&\frac{\partial_{p_3}\Bigl(p_3 (1- i \kappa \omega(p_3)) \Bigr)}{(p_3 + E_n - i \omega(p_3) \kappa p_3)^2(p_3 + E_k - i \omega(p_3) \kappa p_3)} 
\end{eqnarray}
Function $\omega$ may be chosen as follows:
\begin{eqnarray}
	&&\omega_{+}(p_3) =   -\epsilon/2 + \sqrt{\Bigl(p_3 - (\mu - (l+1/2)B/m)\Bigr)^2 + \epsilon^2},\nonumber \\ && {\rm if}\, (\mu - (l+1/2)B/m) - \epsilon \le p_3 \le (\mu - (l+1/2)B/m)+\epsilon  \nonumber
\end{eqnarray}
and
\begin{eqnarray}
	\omega_{+}(p_3) &=&  -\epsilon/2,  \nonumber\\&&{\rm if}\, p_3 < (\mu - (l+1/2)B/m)-\epsilon \nonumber\\&& {\rm or} \quad 
		p_3 > (\mu - (l+1/2)B/m)+\epsilon \nonumber\\ 
	\omega_-(p_3)& =& - \epsilon/2
\end{eqnarray}
One can see that the straight pieces of $\omega_\pm$ cancel each other. Integration over $p_3$ gives
\begin{eqnarray}
	N^{\omega_+(l)}_3 &=&  2\pi i \,\frac{\epsilon_{ij}}{ A }\sum_{k}\int dp_3\frac{1}{(E_k - E_l )^2}\nonumber\\&&\langle l | [\hat{H},\hat{x}_i]|k\rangle \langle k | [\hat{H},\hat{x}_j]|l\rangle  \theta (-E_l)\theta(E_k)
\end{eqnarray}
and 
\begin{eqnarray}
	N^{\omega_- (l)}_3 &=& - 2\pi i \,\frac{\epsilon_{ij}}{ A }\sum_{n,k}\int dp_3\frac{1}{(E_k - E_n )^2}\nonumber\\&&\langle n | [\hat{H},\hat{x}_i]|k\rangle \langle k | [\hat{H},\hat{x}_j]|n\rangle  \theta (-E_n)\theta(E_k)
\end{eqnarray}
We arrive at 
\begin{equation}
	N_3^{\omega_+(l)} =  \Theta( - E_l(B,m))
\end{equation}
and 
\begin{equation}
	N_3^{\omega_-(l)} =  - \sum_n \Theta( - E_n(B,m))
\end{equation}
Thus we obtain
\begin{eqnarray}
	&&N_3^{(l)} = \Theta( - E_l(B,m)) +   \sum_n \Theta( - E_n(B,m)) = \label{Nie}\\&& =  \Theta(\mu - (2l+1) B/(2m)) +  \Bigl[\frac{\mu - B/(2m)}{B/m}\Bigr] \theta(\mu - B/(2m))\nonumber
\end{eqnarray}

\section{Other variations of the model}

\subsection{A model with $M=1$}

We can modify the model considered above in several ways. First of all, let us consider the system with Dirac operator of the form
\begin{eqnarray}
	\hat{Q} &=& i \kappa \hat{p}_4 \Bigl[\frac{\hat{p}_1^2 + (\hat{p}_2 - \hat{x}_1 B)^2  }{2m} - \mu\Bigr] - \hat{p}_3 \nonumber\\&&-  \frac{\Bigl(\hat{p}_1^2 + (\hat{p}_2 - \hat{x}_1 B)^2 \Bigr) }{2m} + \mu
\end{eqnarray}
with parameters $\kappa$, $m$, $\mu$, and $B$. The following consideration repeats the one presented above, and we arrive at the expression for the topological invariant $N_3^{} = N_3^{\omega_+} - N_3^{\omega_-}$, 
where 
\begin{eqnarray}
&&	N^{\omega}_3 = \frac{\epsilon_{ij}}{2 A}\sum_{n,k}\int dp_3\langle n | [\hat{H},\hat{x}_i]|k\rangle \langle k | [\hat{H},\hat{x}_j]|n\rangle \nonumber\\&&\frac{(1-i\omega(p_3) \kappa)^2 \partial_{p_3}(p_3 - i \kappa E_n \omega(p_3))}{(p_3 + E_n - i \omega(p_3) \kappa E_n)^2(p_3 + E_k - i \omega(p_3) \kappa E_k)}
\end{eqnarray}
with 
\begin{equation}
	\hat{H} = \frac{\Bigl(\hat{p}_1^2 + (\hat{p}_2 - \hat{x}_1 B)^2 \Bigr) }{2m} - \mu, \quad \hat{H}|n\rangle = E_n |n\rangle
\end{equation}
We can calculate $N_3^\omega$
integrating over $p_3$ (via the second order residue at $p_3 + E_n - i \omega(p_3) \kappa E_n=0$ ):  
\begin{eqnarray}
	N^{\omega}_3 &=&  2\pi i {\rm sign}\,\omega\,\frac{\epsilon_{ij}}{ A }\sum_{n,k}\int dp_3\frac{1}{(E_k - E_n )^2}\nonumber\\&&\langle n | [\hat{H},\hat{x}_i]|k\rangle \langle k | [\hat{H},\hat{x}_j]|n\rangle  \theta (-E_n)\theta(E_k)
\end{eqnarray}
 The result is given by 
\begin{equation}
	N_3^\epsilon = {\rm sign}\,\omega\,\sum_n \Theta( - E_n(B,m)),
\end{equation}
where $E_n$ is the energy of the $n$ - th Landau level 
\begin{equation}
	E_n(B,m)  = \frac{B}{m} (n+1/2) -\mu, \quad n = 0,1,...
\end{equation}
And we arrive at the same expression as for the above considered model 
$$
N_3^{} = 2\Bigl[\frac{\mu - B/(2m)}{B/m}\Bigr] \theta(\mu - B/(2m))
$$
\thispagestyle{empty}
The Groenewold equation in this case rececives the form
($G = \bar{G}e^{2i(p_2/B - x_1)p_1} $):
\begin{equation}
	\Bigl((B^2 \partial_{p_1}^2 + \partial_{x^1}^2  + 8m \mu)(1-i \kappa p_4) - 8m  p_3\Bigr) \bar{G} = 8m  e^{-2i(p_2/B - x_1)p_1}
\end{equation}
Solution of this equation gives
\begin{eqnarray}
	&&{G}_W(x_1,p_1,p_2,p_3,p_4) =- \frac{2m}{\pi } e^{2i(p_2/B - x_1)p_1} \times \nonumber\\&& \int \frac{e^{-i\gamma (x_1 - p_2/B) - i \xi p_1 - i \xi \gamma/2}}{(B^2\xi^2 + \gamma^2 - 8m \mu)(1-ip_4 \kappa)  + 8m  p_3 }d\gamma d\xi \label{GW1}
\end{eqnarray}
In order to determine the positions of Fermi surfaces we use the Landau level representation 
\begin{eqnarray}
&&	G_W(x_1,p_1,p_2,p_3,p_4) = \sum_n \int dy e^{ip_1 y}\nonumber\\&&\frac{\Psi_n(x_1 - y/2 - p_2/B) \bar{\Psi}_n(x_1 + y/2 - p_2/B)}{- p_3 - (\frac{B}{m}(n+1/2) - \mu)(1-i \kappa p_4)}
\end{eqnarray}
The singularities of the above expresion give the position of the Fermi surface that coincides with the one of the original model  
\begin{equation}
	p_4 = 0, \quad p_3 = \mu - \frac{B}{m}(n+1/2), n = 0, 1, ...  
\end{equation}
As above, we can also  define quantities $N_3^{(i)}$ that are given by integrals along the hypertubes surrounding the disconnected pieces of the Fermi surface. We arrive then at the same expression of Eq. (\ref{Nie}).

\subsection{A model with topological invariant protected by symmetry ($M=4$)}

Let us consider the matrix extension of the model with the Dirac operator of the form
\begin{eqnarray}
	\hat{Q} &=& i \kappa \hat{p}_4 \Bigl(\hat{p}_1 \gamma^0\gamma^1 + (\hat{p}_2 - \hat{x}_1 B) \gamma^0 \gamma^2+i \mu \gamma^0 \gamma^3 \Bigr)\nonumber\\&&- i\hat{p}_3\gamma^0 \gamma^3  - \hat{p}_1 \gamma^0\gamma^1\nonumber\\&& - (\hat{p}_2 - \hat{x}_1 B) \gamma^0 \gamma^2-i\mu \gamma^0 \gamma^3 
\end{eqnarray}
with parameters $\kappa$ and $B$ and ordinary gamma - matrices $\gamma^i$ taken in chiral representation.
 One may define the corresponding topological invariant protected by symmetry  with $\hat{T} = \gamma^5$. It can be calculated for $p_4 =  \omega_\pm $:
  $$
 N_3^{(\gamma^5)} = N_3^{\omega_+} - N_3^{\omega_-}
 $$ 
 where 
 \begin{eqnarray} 
 	N^{\omega}_3&	=&{-}\frac{1}{V \,24\pi^2}\int d^3 x\int_{p_4 = \omega} \text{tr}_{D}\Bigl(\gamma^5{G}_W\star d{Q}_W\star \wedge \nonumber\\&& d{G}_W\star\wedge d{Q}_W \Bigr) \label{Ni2}
 \end{eqnarray}
  Using the same  machinery as above we arrive at
 \begin{eqnarray}
 	&& N^{\epsilon}_3 = 2\frac{\epsilon_{ij}}{2 A}\sum_{n,k}\int dp_3\langle n | [\hat{H},\hat{x}_i]|k\rangle \langle k | [\hat{H},\hat{x}_j]|n\rangle \nonumber\\&&\frac{(1+i E_n \kappa \partial_{p_3}\omega)(1-i \omega \kappa)^2}{(p_3 - E_n + i E_n  \omega \kappa )^2(p_3 - E_k + i E_n \omega \kappa )}
 \end{eqnarray}
 with 
 \begin{equation}
 	\hat{H} =  i \sigma^3 \sigma^1 \hat{p}_1 + i \sigma^3 \sigma^2  (\hat{p}_2 - \hat{x}_1 B) - \mu, \quad \hat{H}|n\rangle = E_n |n\rangle
 \end{equation}
 As in the previous case we obtain after integration over $p_3$
 \begin{eqnarray}
 	&& N^{\epsilon}_3 =  2\pi i {\rm sign}\,\epsilon\,\frac{\epsilon_{ij}}{ A}\sum_{n,k}\int dp_3\frac{1}{(E_k - E_n )^2}\nonumber\\&& \langle n | [\hat{H},\hat{x}_i]|k\rangle \langle k | [\hat{H},\hat{x}_j]|n\rangle  \theta (-E_n)\theta(E_k)
 \end{eqnarray}

  The result is given by 
\begin{equation}
	N_3^\omega = 2\, {\rm sign}\,\omega\,\sum_n \Theta(E_n(B,\mu)),
\end{equation}
where $E_n$ is the energy of the $n$ - th Landau level 
\begin{equation}
	E_n(B,\mu)  = \pm \sqrt{2B n} -\mu, \quad n = 0,1,...
\end{equation}
The obtained expression for $N_3^{\gamma^5}$ is divergent in ultraviolet: 
\begin{equation}
	N_3^{\gamma^5} = 4\, \sum_n \Theta(E_n(B,\mu)),\label{N3g5}
\end{equation}
The situation with this divergency is similar to the one of the quantum Hall effect in graphene. Formally the corresponding expression obtained using the above mentioned machinery applied to the low energy continuum model is given by Eq. (\ref{N3g5}) multiplied by the inverse Klitzing constant. Of course, the experiment shows a different result. Namely, the QHE conductivity is vanishing at half filling ($\mu = 0$). 
\thispagestyle{empty}

The explanation for this puzzle is that the proper ultraviolet regularization subtracts the contribution of Landau levels with negative $E_n$. At the same time the half of the contribution of the LLL ($E_0 =0$) is subtracted. Technically the subtraction is achieved authomatically, when proper regularization is added. Say, lattice regularization modifies expression of Eq. (\ref{N3g5}) at large values of $n$: the corresponding Landau levels contribute with their Chern numbers that differ from $1$. In particular, at certain negative values of $n$ the contributions are large and negative, so that at $\mu = 0$ the resulting expression is precisely zero. The Pauli - Villars regularization gives much more transparent solution. Namely, the contributions of Pauli - Villars regulators with large mass cancel one by one all contributions to $N_3^{\gamma^5}$ of Landau levels with $E_n < 0$, while only half contribution of $E_0$ is cancelled. 

Thus we come to expression 
  \begin{equation}
  	N_3^{\gamma^5} = \Bigl(4\, \Bigl[\frac{\mu^2}{2B}\Bigr] + 2\Bigr)\,{\rm sign}\,\mu  \label{N3g5_}
  \end{equation} 

\subsection{Models with curved Fermi surfaces}
\subsubsection{A model with cylindrical  Fermi surface }

Let us consider another modification of the model, in which the Fermi surfaces are already not planes $p_3 = const$ but have cylindrical  form. We start from the Dirac operator 
\begin{equation}
	\hat{Q} = i \kappa \lambda \hat{p}_4 (\hat{H}-\mu \gamma^5) - \hat{{p}}_r - (\hat{H}  - \mu \gamma^5)\lambda 
\end{equation}
Here $p_r = \sqrt{p_x^2+p_y^2}$ is radial component of momentum. 
It is assumed that $\hat{H}$ commutes with $\gamma^5$. $\kappa$ and $\lambda$ are parameters. The Wigner transformed Green function is assumed to have the form
\begin{eqnarray}
&&	G_W(x_1,p_1,p_2,p_3,p_4)  = \sum_{nk\pm} \int d^3y e^{i\bar{p} \bar{y}}\times \nonumber\\ && \times \frac{\Psi_{nk\pm}(\bar{x} - \bar{y}/2 ) \bar{\Psi}_{nk\pm}(\bar{x} + \bar{y}/2 )}{ - {{p}_r} \mp \lambda({\cal E}_n - \mu)(1-i p_4 \kappa)}
\end{eqnarray}
where ${\cal E}_n$ are (positive chirality) eigenvalues while $\Psi_{nk\pm}$ are eigenfunctions of the Hamiltonian $\hat{H}$ corresponding to positive (negative chirality). In order to define the Hamiltonian $\hat{H}$ we pass to the new coordinates in momentum space. Namely, let $(p_r, p_z ,\phi)$ be the cylindrical coordinates in momentum space. We define the frame $(p_r\in (0,\infty), p_z \in (-\pi/b, + \pi/b), p_\phi = \phi/a\,  \in (-\pi/a,  \pi/a )$. For example, $d^3 p =a  p_r dp_r dp_z dp_\phi$. We assume that parameters $b,a \to \infty$. We define
\begin{eqnarray}
	\hat{H}& =& f_a(p_\phi +  B \hat{x}_z)\gamma^0\gamma^1 +  f_b(p_z) \gamma^0\gamma^2  
\end{eqnarray}
with $f_a(p) = \frac{1}{a}{\rm sin}\,pa + \frac{1}{a}(1-{\rm cos} \,pa)$, which gives
\begin{eqnarray}
	\hat{H}& \approx & (p_\phi +  B \hat{x}_z)\gamma^0\gamma^1 +  p_z \gamma^0\gamma^2  
\end{eqnarray}
with $\hat{x}_z = i \partial_{p_z}$ and $\hat{x}_\phi = i \partial_{p_\phi}$. 
We also denote 
\begin{equation}
	\hat{\cal H} = (p_\phi +  B \hat{x}_z)\sigma^1 +  p_z \sigma^2 \label{ham0}
\end{equation}
\thispagestyle{empty}
Then $p_r$ commutes with Hamiltonian, and spectrum of this Hamiltonian for any $p_r$ is: 
\begin{equation}
	\hat{\cal H} |n, k\rangle = {\cal E}_n |n, k\rangle
\end{equation}
with ${\cal E}_n =  \sqrt{2B|n|} \,{\rm sign}\,n$. Each energy level is degenerate, the degenerate states are enumerated by the admitted values of $p_\phi = p^{(k)}_\phi$. These are the values that obey $e^{i p^{(k)}_\phi L_\phi}  = 1$, and maximal possible value of $p^{(k)}_\phi$ is $ B L_z$ (where $L_\phi$ is maximal value of coordinate $x_\phi$, while $L_z$ is the size of the system in z - direction). Therefore, $p^{(k)}_\phi = { 2\pi k/L_\phi}$ and $k_{max} =\frac{B L_\phi L_z}{2\pi}\, $. The Hamiltonian of the right  - handed particles is equal to that of the left - handed ones with the minus sign. The degeneracy of each level is equal to $N=k_{max}$. We denote by $A = L_\phi L_z$ the area of coordinate space in coordinates $x_z,x_\phi$.

Taking this in mind we calculate the expression for $N^{(\gamma^5)}_3$ as follows
$$
N_3^{(\gamma^5)} = N_3^{+\epsilon} - N_3^{-\epsilon}
$$ 
where 
\begin{eqnarray} 
	N^{\epsilon}_3&	= &{-}\frac{1}{V \,24\pi^2}\int d^3 x\int_{p_4 = \epsilon} \text{tr}_{D}\Bigl(\gamma^5{G}_W\star d{Q}_W\nonumber\\&&\star \wedge d{G}_W\star\wedge d{Q}_W \Bigr) \label{Ni2l}
\end{eqnarray}
As proposed in the main text we represent Eq. (\ref{Ni2l}) in the parametrization of the hypersurface $p_4=\epsilon$ by real numbers $\bar{k} = (k_1,k_2,k_3) = (p_r,p_\phi,p_z)$.  We express $\bar{p}(\bar{k})$ through the new parameters $\bar{k}$. In terms of the latter the necessary   representation reads 
\begin{align}
	{N}^{\epsilon}
	&=\frac{\epsilon_{ijk}}{24 \pi^2 }
	\int_{\Sigma^{(i)}}d^3 k
	\int   \frac{d^3 \xi}{{ V}}
	\tr \Bigl[\hat{\gamma}^5
	\tilde{G}\circ \partial_{k_i} \tilde{ Q} \circ\nonumber\\& \tilde{ G}
	\circ \partial_{k_j} \tilde{ Q}\circ \tilde{ G} \circ  \partial_{k_k} \tilde{ Q}
	\Bigr]\label{Ncompl0}
\end{align}
with 
\begin{align}
	\circ &= e^{\frac{i}{2}\Bigl(\overleftarrow{\partial_{\xi^i}}\overrightarrow{\partial_{k_i}} - \overleftarrow{\partial_{k_i}}\overrightarrow{\partial_{\xi^i}} \Bigr)}\label{eqo}
\end{align}
and  $
{ V} = \int d^3 \xi
$.
Correspondingly, the limit of infinitely large $ V$ in Eq. (\ref{Ncompl0})  is to be considered. 
Vector $\bar{\xi} = (x_r,x_\phi,x_z)$ represents the new parametrization of coordinate space. These new coordinates are determined by equation 
$
\frac{\partial \xi^i(\bar{k},\bar{x})}{\partial x^j} = \frac{\partial p_j(\bar{k})}{\partial k_i}
$.
Therefore, 
$
\xi^i =\frac{\partial p_j(\bar{k})}{\partial k_i} x^j \, \quad (i,j = 1,2,3)
$.
Correspondingly, $\int d^3 \xi = {\rm Det}\,\frac{\partial p(\bar{k})}{\partial k}\, \int d^3 x$. 

By $\tilde Q$ in Eq. (\ref{Ncompl0}) we understand 
\begin{align}
	\tilde{Q}(\bar{k},\bar{\xi}) \equiv  Q((\bar{p}(\bar{k}),\epsilon)),x(\bar{k},\bar{\xi})) \label{B}
\end{align}
with $x^j = (\frac{\partial k_k}{\partial p_j} \, \xi^k)$, ($i,j = 1,2,3$).
Here there is no dependence on $x^4$ because we consider the equilibrium system, while 
$p = (\bar{p}(\bar{k}), \epsilon)$.

Correspondingly, we have
\begin{equation}
	\tilde{Q} = i \kappa \lambda \epsilon ({H}-\mu \gamma^5) - \hat{{p}}_r - ({H}  - \mu \gamma^5)\lambda 
\end{equation}
with 
\begin{eqnarray}
	{H}& \approx & (p_\phi +  B {x}_z)\gamma^0\gamma^1 +  p_z \gamma^0\gamma^2  
\end{eqnarray}
and in original coordinates 
\begin{eqnarray}
	{H}& \approx & (\frac{1}{a}{\rm Arctg}\, p_2/p_1 +  B x_3)\gamma^0\gamma^1 +  p_3 \gamma^0\gamma^2  
\end{eqnarray}

By $\tilde{G}$ we then understand the function inverse to $\tilde{Q}$ with respect to the $\circ$ product: 
\begin{align}
	\tilde{Q} \circ \tilde{G} = 1\label{C}
\end{align}
The standard calculation methods then lead us to 
\begin{eqnarray}
	N^{\epsilon}_3 &=& \sum_\pm (\pm \lambda^2) \frac{\epsilon_{ij}}{2 A}\sum_{n_1,n_2,k_1,k_2}\int_0^{\infty} dp_r\langle n_1,k_1 | [\hat{\cal H},\hat{\xi}_i]|n_2,k_2\rangle  \nonumber\\&&\frac{\langle n_2,k_2 | [\hat{\cal H},\hat{\xi}_j]|n_1,k_1\rangle}{(p_r \pm E_{n_1}(1 - i \epsilon \kappa))^2(p_r \pm E_{n_2}(1 -i \epsilon \kappa))}
\end{eqnarray}
with $E_n = \lambda({\cal E}_n - \mu)$.  Correspondingly, indexes $i,j = 2,3 = "\phi", "z"$.
We may rewrite this expression with the integral over $p_r$ within $(-\infty, +\infty)$:
\begin{eqnarray}
	N^{\epsilon}_3 &=&   \lambda^2 \frac{\epsilon_{ij}}{2 A}\sum_{n_1,n_2,k_1,k_2}\int_{-\infty}^{+\infty} dp_r\langle n_1,k_1 | [\hat{\cal H},\hat{\xi}_i]|n_2,k_2\rangle  \nonumber\\&&\frac{\langle n_2,k_2 | [\hat{\cal H},\hat{\xi}_j]|n_1,k_1\rangle}{( p_r + E_{n_1}(1 - i \epsilon \kappa))^2( p_r + E_{n_2}(1 -i \epsilon \kappa))}
\end{eqnarray} 
We consider the limit $\epsilon  \to \pm 0$, and perform integration over $p_r$ 
\begin{eqnarray}
	&& N^{\epsilon}_3 =  2\pi i  {\rm sign}\,\epsilon\,\frac{\epsilon_{ij}}{ A}\sum_{n_1,n_2,k_1,k_2}\frac{1}{({\cal E}_{n_2} - {\cal E}_{n_1} )^2}\\&&\langle n_1,k_1 | [\hat{\cal H},\hat{\xi}_i]|n_2,k_2\rangle \langle n_2,k_2 | [\hat{\cal H},\hat{\xi}_j]|n_1,k_1\rangle  \theta (-E_{n_1})\theta(E_{n_2})\nonumber
\end{eqnarray}

The result is given by 
\begin{equation}
	N_3^\epsilon = {\rm sign}\,\epsilon\,\sum_{n} \Theta( - E_n),
\end{equation}
One can see that $N_3^{-\epsilon} = - N_3^{+\epsilon}$, and we arrive at 
$$
N_3^{(\gamma^5)} = 2 \sum_{n} \Theta(\mu - \sqrt{2 B |n|} \, {\rm sign}\, n)
$$
As in the previous example, this expression is divergent, but being regularized, it gives
$$
N_3^{(\gamma^5)} = 2 \, {\rm sign}\,(\mu)\, \Bigl(1/2+\sum_{n>0} \Theta(\mu - \sqrt{2 B |n|} )\Bigr)
$$

 In this case the Fermi surfaces have the form of cylinders (with axis z) and radii 
 \begin{equation}
 		p_4 = 0, \quad |p_r| = \mp \lambda(\mu - {\rm sign}\,(n)\, \sqrt{2 B |n|}), n = 0, \pm 1, ...  
 \end{equation}
(Only those values of $n$ contribute, for which the right hand side of this expression is not negative.)
The particular interesting case corresponds to $\mu = \delta$, $\delta \to 0$. Then the only Fermi surface shrinks to cylinder with very small radius. The corresponding invariant $N_3^{(\gamma^5)} = {\rm sign }\, \delta$ protects this Fermi surface.  

\subsubsection{A model with spherical Fermi surface }

The modification of the model with spherical Fermi surface follows closely the consideration of the previous subsection. Again, we start from the Dirac operator 
\begin{equation}
	\hat{Q} = i \kappa \lambda \hat{p}_4 (\hat{H}-\mu \gamma^5) - \hat{{p}}_r - (\hat{H}  - \mu \gamma^5)\lambda 
\end{equation}
but now $p_r = \sqrt{p_x^2+p_y^2+p_z^2}$ is radial component of momentum. 
In order to define the Hamiltonian $\hat{H}$ we pass to the spherical coordinates in momentum space. Namely, let $(p_r, \theta ,\phi)$ be the spherical coordinates in momentum space. We define the frame $(p_r\in (0,\infty), p_\theta = \theta/b \in (0, + \pi/b), p_\phi = \phi/a\,  \in (-\pi/a,  \pi/a )$. For example, $d^3 p =a b  p_r {\rm sin}(b p_\theta) dp_r dp_\theta dp_\phi$. As above we assume that parameters $b,a \to \infty$, and define
\begin{eqnarray}
	\hat{H}& =& f_a(p_\phi +  B \hat{x}_\theta)\gamma^0\gamma^1 +  p_\theta \gamma^0\gamma^2  
\end{eqnarray}
with $f_a(p) = \frac{1}{a}{\rm sin}\,pa + \frac{1}{a}(1-{\rm cos} \,pa)$, which gives
\begin{eqnarray}
	\hat{H}& \approx & (p_\phi +  B \hat{x}_\theta)\gamma^0\gamma^1 +  p_\theta \gamma^0\gamma^2  
\end{eqnarray}
with $\hat{x}_\theta = i \partial_{p_\theta}$ and $\hat{x}_\phi = i \partial_{p_\phi}$.

The further calculation is identical to the one for the case of cylindrical Fermi surface. 

 We arrive at
$$
N_3^{(\gamma^5)} = 2 \, {\rm sign}\,(\mu)\, \Bigl(1/2+\sum_{n>0} \Theta(\mu - \sqrt{2 B |n|} )\Bigr)
$$

In this case the Fermi surfaces have the form of spheres with radii 
\begin{equation}
	p_4 = 0, \quad |p_r| = \mp \lambda(\mu - {\rm sign}\,(n)\, \sqrt{2 B |n|}), n = 0, \pm 1, ...  
\end{equation}
(Only those values of $n$ contribute, for which the right hand side of this expression is not negative.)
In the case $\mu = \delta$, $\delta \to 0$ the only Fermi surface shrinks to sphere with very small radius. The corresponding invariant $N_3^{(\gamma^5)} = {\rm sign }\, \delta$ protects it.

\thispagestyle{empty}

\bibliography{wigner3,cross-ref,biblio_corrected} 
%\printbibliography
\end{document}
